# Supplementary material for: WITCHER : Detecting Crash Consistency Bugs in Non-volatile Memory Programs
Source: arXiv:2012.06086 source file (2020-12-11)
Supplement: Supplementary file 1 [file appendix.tex]

%%%%%%%%%
\section*{Appendix}

%%%%%%%%%%%
\section{Details on New Bugs Found}
\label{s:appendix:newbugs}

\autoref{t:bugs} shows the list of crash consistency bugs detected by
\sys from \NumOfAppsBugDetected NVM programs. For each bug, we provide program
name (the total number of bugs), bug ID, novelty (new vs. old), source
code location, bug type (ordering vs. atomicity), description, bug
impact, and fix strategy. We now discuss their fix strategies in more
detail.

\begingroup
% \addtolength{\tabcolsep}{-3pt}
 % Default value: 1
\begin{table*}[bt]
  \centering
  \resizebox{1\textwidth}{!}{%\begin{tabular}{l|c|llllccc}

\begin{tabular}{l|c|ccclll}
\hline
\textbf{App (Total \#Bugs)} & \textbf{Bug ID} & \textbf{New} &
\textbf{Code} & \textbf{Type} & \textbf{Description} & \textbf{Impact}
& \textbf{Fix strategy}  \\ \hline
WOART (1)          & 1  & \yesmark & \cite{woart-bug-0}     & PA & Atomicity in node split                  & Inconsistent structure & inconsistency-recoverable design                      \\ \hline
FAST-FAIR (3)      & 2  & \yesmark & \cite{ff-bug-0}        & PO & Missing persistence primitives           & Lost key-value         & add persistence primitives                            \\
                   & 3  & \yesmark & \cite{ff-bug-1}        & PA & Partial inconsistency is never recovered & Inconsistent structure & inconsistency-recoverable design                      \\
                   & 4  & \nomark  & \cite{ff-bug-2}        & PA & Atomicity in node splitting              & Inconsistent structure & logging/transaction                                   \\ \hline
Level Hashing (17) & 5  & \yesmark & \cite{lh-bug-0}        & PO & Incorrect persistence order              & Unexpected key-value   & persistence reorder~\cite{lh-commit}                  \\
                   & 6  & \yesmark & \cite{lh-bug-1}        & PO & Incorrect persistence order              & Unexpected key-value   & persistence reorder~\cite{lh-commit}                  \\
                   & 7  & \yesmark & \cite{lh-bug-2}        & PO & Incorrect persistence order              & Unexpected key-value   & persistence reorder~\cite{lh-commit}                  \\
                   & 8  & \yesmark & \cite{lh-bug-6}        & PO & Incorrect persistence order              & Unexpected key-value   & persistence reorder~\cite{lh-commit}                  \\
                   & 9  & \yesmark & \cite{lh-bug-7}        & PO & Incorrect persistence order              & Unexpected key-value   & persistence reorder~\cite{lh-commit}                  \\
                   & 10 & \yesmark & \cite{lh-bug-9}        & PO & Incorrect persistence order              & Unexpected key-value   & persistence reorder~\cite{lh-commit}                  \\
                   & 11 & \yesmark & \cite{lh-bug-11}       & PO & Incorrect persistence order              & Unexpected key-value   & persistence reorder~\cite{lh-commit}                  \\
                   & 12 & \yesmark & \cite{lh-bug-13}       & PO & Incorrect persistence order              & Unexpected key-value   & persistence reorder~\cite{lh-commit}                  \\
                   & 13 & \yesmark & \cite{lh-bug-14}       & PO & Incorrect persistence order              & Unexpected key-value   & persistence reorder~\cite{lh-commit}                  \\
                   & 14 & \yesmark & \cite{lh-bug-15}       & PO & Incorrect persistence order              & Unexpected key-value   & persistence reorder~\cite{lh-commit}                  \\
                   & 15 & \yesmark & \cite{lh-bug-4}        & PA & Atomicity in rehashing                   & Inconsistent structure & logging/transaction                                   \\
                   & 16 & \yesmark & \cite{lh-bug-5}        & PA & Atomicity in rehashing                   & Inconsistent structure & logging/transaction                                   \\
                   & 17 & \yesmark & \cite{lh-bug-8}        & PA & Atomicity between two metadata           & Duplicated key-value   & inconsistency-tolerable design                        \\
                   & 18 & \yesmark & \cite{lh-bug-10}       & PA & Atomicity between two metadata           & Duplicated key-value   & inconsistency-tolerable design                        \\
                   & 19 & \yesmark & \cite{lh-bug-12}       & PA & Atomicity between two metadata           & Duplicated key-value   & inconsistency-tolerable design                        \\
                   & 20 & \yesmark & \cite{lh-bug-3}        & PA & Atomicity between two metadata           & Lost key-value         & merge to word size~\cite{lh-commit}                   \\
                   & 21 & \yesmark & \cite{lh-bug-16}       & PA & Atomicity between two metadata           & Lost key-value         & merge to word size~\cite{lh-commit}                   \\ \hline
CCEH (2)           & 22 & \nomark  & \cite{cceh-bug-0}      & PA & Atomicity in rehashing                   & Inconsistent structure & inconsistency-recoverable design                      \\
                   & 23 & \yesmark & \cite{cceh-bug-1}      & PA & Partial inconsistency is never recovered & Unexpected op failure  & inconsistency-recoverable design                      \\ \hline
P-ART (2)          & 24 & \yesmark & \cite{part-bug-0}      & PA & Atomicity between metadata and key-value & Inconsistent structure & inconsistency-tolerable design~\cite{recipe-commit-1} \\
                   & 25 & \yesmark & \cite{part-bug-1}      & PA & Atomicity between metadata and key-value & Inconsistent structure & inconsistency-tolerable design~\cite{recipe-commit-1} \\ \hline
P-BwTree (2)       & 26 & \yesmark & \cite{pbwtree-bug-0}   & PO & Missing persistence primitives           & Inconsistent structure & add persistence primitives                            \\
                   & 27 & \yesmark & \cite{pbwtree-bug-1}   & PO & Missing persistence primitives           & Inconsistent structure & add persistence primitives                            \\ \hline
P-CLHT (1)         & 28 & \yesmark & \cite{pclht-bug-0}     & PO & Missing persistence primitives           & Lost key-value         & add persistence primitives~\cite{recipe-commit-0}     \\ \hline
P-HOT (3)          & 29 & \yesmark & \cite{phot-bug-0}      & PO & Missing persistence primitives           & Inconsistent structure & add persistence primitives~\cite{recipe-commit-0}     \\
                   & 30 & \yesmark & \cite{phot-bug-1}      & PO & Missing persistence primitives           & Inconsistent structure & add persistence primitives~\cite{recipe-commit-0}     \\
                   & 31 & \yesmark & \cite{phot-bug-2}      & PO & Missing persistence primitives           & Inconsistent structure & add persistence primitives~\cite{recipe-commit-0}     \\ \hline
P-Masstree (1)     & 32 & \yesmark & \cite{pmasstree-bug-0} & PA & Atomicity in node splitting              & Inconsistent structure & logging/transaction                                   \\ \hline
Array (1)          & 33 & \nomark  & \cite{array-bug-0}     & PA & Atomicity between metadata and value     & Inconsistent structure & logging/transaction                                   \\ \hline
B-Tree (2)         & 34(*) & \yesmark & \cite{btree-bug-0}  & PO & Incorrect persistence order in PMDK      & Inconsistent structure & persistence reorder~\cite{btree-issue-0}              \\
                   & 35 & \nomark  & \cite{btree-bug-1}     & PA & Missing logging in a transaction         & Inconsistent structure & add logging                                           \\ \hline
RB-Tree            & 36 & \nomark  & \cite{rbtree-bug-0}    & PA & Missing logging in a transaction         & Inconsistent structure & add logging                                           \\ \hline
Hashmap-TX         & 37 & \yesmark & \cite{hash-bug-0}      & PO & Use-after-free                           & Unexpected op failure  & copy before free                                      \\ \hline
\end{tabular}
}

  \vspace{.5em}
  \scriptsize
  NOTE: \quad
  \textbf{PO}: persistence ordering bugs \quad
  \textbf{PA}: persistence atomicity bugs \quad
  \textbf{(*)}: Bug in the PMDK library
  \vspace{6pt}
  \caption{
  List of bugs discovered by \sys in the tested persistent applications
  in~\autoref{t:bugstats}.
  % The total number of bugs reported is 32.
  All \NumOfTotalBugs bugs have been confirmed by authors, and \NumOfNewBugs of
  \NumOfTotalBugs bugs are new. There are \NumOfOrderBugs persistence ordering bugs and 
  \NumOfAtomicityBugs persistence atomicity bugs. One bug (ID 34) is in the PMDK library.
  }
  %\vspace{-15px}
\label{t:bugs}
\end{table*}
\endgroup

\PP{Fixing persistence ordering bug}
\sys detected \NumOfOrderBugs persistence ordering bugs in total. 

\squishlists

\item
7 of \NumOfOrderBugs
persistence ordering bugs occurred because developers did not add
persistence primitives or passed incorrect addresses as
parameters. Fixing these bugs is straightforward: adding required
persistence primitives (\flush and/or \fence) or passing the correct
address parameter.
So-called missing persistence primitive bugs (discussed in
XFDetector~\cite{xfdetector-liu-asplos20} and RECIPE~\cite{recipe-lee-sosp19})
belong to this category.

\item
The rest 12 persistence ordering bugs had persistence primitives, but
they persist multiple stores in an incorrect order. Fixing them
requires reordering persistence primitives. For example, to fix the
persistence ordering bug (Bug ID 5) in \cc{level_insert} function
in~\autoref{f:lh-bugs}(b), as confirmed by the
authors~\cite{lh-commit}, the key and value should be persisted before
updating the token, so Lines~\lhinsertpflushk-\lhinsertfencekv~should
be moved before updating the token at Line~\lhinserttoken.
The bug (Bug ID 34) in PMDK's persistent pool/heap allocation function
\cc{pmemobj\_tx\_zalloc}~\cite{btree-issue-0} was also fixed by reordering
source codes.

\squishends

\PP{Fixing persistence atomicity bug}
%\TODO{now we have missing logging in TX-based program now}
%
\sys detected \NumOfAtomicityBugs persistence atomicity bugs in total. 
Two cases (Bug IDs 35 and 36) were a missing logging problem in transactional
programs B-Tree and RB-Tree. Fixing is relatively trivial -- just add a
logging.
However, things are more complex for rest 17 bugs appeared in low-level NVM
programs.  Due to the lack
of persistence atomicity primitives, all of them indeed required
design or implementation-level changes. We observed the following
four fixing strategies from the developers:

\squishlists

\item
To merge multiple writes into \emph{one word-size write} within one
cache line to guarantee atomicity~\cite{intel:sdm}.
For example, to fix the persistence atomicity bug in \cc{level_update}
function (\autoref{f:lh-bugs}(c)), the authors~\cite{lh-commit} merged
all tokens in a bucket into a single word by modifying the structure
layout. The patched code now uses a single store instruction to update
two tokens atomically.

\item
To make program \emph{crash-inconsistency-tolerable}.
The key insight of the crash-inconsistency-tolerable design is similar
to the concurrent data structure's \emph{helping
mechanism}~\cite{help-censorhillel-podc15}, where an operation started
by one thread but failed is later completed by another
thread. Similarly, a crash-inconsistency-tolerable design asks an
operation that notices an inconsistent state to fix it on behalf.
For Bugs 17-19 leading to duplicated key-value in Level
Hashing, the developers suggested a solution that checks and removes the
duplicates in delete and update operations. %The fix has not yet been
%committed at the time of this submission.
%%
The two Bugs 24 and 25 from P-ART were fixed by making the
inconsistency visible and letting it fixed by a later
operation~\cite{recipe-commit-1}.

\item
To make program \emph{crash-inconsistency-recoverable}.
Similar to the above crash-inconsistency-tolerable design, this
solution introduces a recovery code which is executed after a crash
and fixes any observed inconsistency. Taking Bug 22 in CCEH as an
example, when incremental rehashing, two metadata (a pointer to the
new bucket and \cc{local_depth} in the old bucket) are not guaranteed
to be atomically persisted. After the discussion with the authors,
they proposed a fix that persists the new bucket pointer before
\cc{local_depth} and uses the recovery mechanism to roll
back the new bucket pointer based on the \cc{local_depth} if needed.
The solutions for Bugs 3 and 23 were similar in spirit.

\item
To use \emph{logging/transaction} techniques.
Logging/transaction can be used to fix persistence atomicity
bugs. However, we found that developers (Level Hashing, CCEH, and
RECIPE) were concerned about using logging due to its high
overhead, and they would prefer avoiding them if any of the above
fixing approaches can be applied. Nonetheless, the Level Hashing
developers suggested that logging may be needed for the atomicity bug
in their \cc{rehashing} operation.

\squishends

%%%%%%%%%%%%
\section{Testing Multi-Threaded NVM Programs}
\label{s:appendix:multithread}

\PP{Design}
%
% Now we discuss how \sys supports multi-threaded NVM programs.
%The core idea is to test a multi-threaded execution in a way that we can
%construct the oracles to compare the output.
Testing a multithreaded NVM program requires two changes in test case generation
and output equivalence checking.
First, the test case should be deterministic (as discussed in \autoref{s:design:tc}). 
Suppose we consider a test case with \cc{N}
operations and \cc{M} threads. We randomly pick the \cc{i}-th
operation, run the ``prefix'' test case from 1st to \cc{(i-1)}-th
operations sequentially, the next \cc{M} (\cc{i}-th to
\cc{(i+M-1)}-th) operations concurrently, and the rest ``suffix'' test
case (after \cc{(i+M)}-th) operations sequentially again. Then, \sys
performs program tracing (\autoref{s:design:trace}) and invariant
inference (\autoref{s:design:invariant}) as usual. The next crash NVM
image generation (\autoref{s:design:ctp}) is only applied to the middle
concurrent testing region as if a crash happens during concurrent
execution. The sequential prefix and suffix parts reflect one
linearizable concurrent execution with deterministic
results to facilitate crash NVM images and oracles generation.

Second, output equivalence checking should compare with more oracles, given
that \cc{M} concurrent operations may crash (as discussed in
\autoref{s:design:multithread}). 
%Recall
%that for single-threaded case, there is one crashing
%operation. However, now we simulate a crash while \cc{M} concurrent
%operations are running. Each operation has two legal states (committed
%or rollbacked), and we also need to consider different
%permutation. Therefore, 
For \cc{M} concurrent operation, the number of oracles is $P(M,0)
+ P(M,1) + ... + P(M,M-1) + P(M,M)$ where $P(m,k) =
\sfrac{m!}{(m-k)!}$. 
%For example, we need 5 oracles for 2 threads and
%65 oracles for 4 threads. We leave oracle optimization as future
%work.

\PP{Results}
We performed multi-threaded testing for FAST-FAIR, CCEH, and
P-ART. Each test case contains 2000 random operations as in the
single-threaded testing. We randomly picked 200 concurrency testing
points and tested them with four threads.
\sys is able to report the same persistence bugs of those data
structures as in~\autoref{t:bugs}, but it does not report a
multi-threading-specific bug. To improve \sys's capability of
detecting multi-threading related crash consistency bugs, we could
extend \sys with (1) a multi-thread test case generator to increase
contention between threads and (2) a thread scheduler to explore more
thread interleaving. We leave them as future works.
